# Supplementary material for: The Tur\'{a}n density of short tight cycles
Source: arXiv:2506.03223 ancillary file (2025-06-03)
Supplement: Supplementary file 1 [file readme.pdf]

## VERIFICATION OF FLAG ALGEBRAS GENERATED RESULTS

### Full verification

The certificates (files with the `.pickle` extension) are generated by the `flag algebras` package in Sage (available at <https://github.com/bodnalev/sage>) using the scripts in the notebooks `no_c5_k4.ipynb` and `no_c7.ipynb`. All these certificates are serialized Python 3 objects.

The verification programs are written in Python 3. The full verification, which takes around 85 hours in a modern personal computer, can be performed by executing the `full-verify` program inside a folder containing all six certificates:

```
$ cd certificates/  
$ python3 full-verify.py
```

The program calls the `validator` and `verifier` programs on each certificate. The calls are made in the following way:

```
$ python3 validator.py prop_3_1_c5k4.pickle  
$ python3 verifier.py prop_3_1_c5k4.pickle
```

### Validate objectives and assumptions

The `validator` program loads a certificate as a Python pickle file and verifies that that the objective function and positivity assumptions of its corresponding proposition are correctly translated into the certificate. Its usage message is the following.

```
usage: validator.py [-h] {prop_3_1_c5k4.pickle,prop_3_1_c7.pickle,  
                        prop_3_2_c5k4.pickle,prop_3_2_c7.pickle,  
                        prop_3_3_c5k4.pickle,prop_3_3_c7.pickle}  
  
Validates that the objectives and assumptions of a given certificate correspond  
to those in the corresponding proposition.  
  
positional arguments:  
  {prop_3_1_c5k4.pickle,prop_3_1_c7.pickle,prop_3_2_c5k4.pickle,  
   prop_3_2_c7.pickle,prop_3_3_c5k4.pickle,prop_3_3_c7.pickle}  
                                path of the pickle file  
  
options:  
  -h, --help            show this help message and exit  
  
examples:  
  $ python validator.py prop_3_1_c5k4.pickle
```

The objective functions and positivity assumptions for each propositions can be found in the following locations.

- Proposition 3.1: Lines 179–186.
- Proposition 3.2: Lines 189–250.
- Proposition 3.3: Lines 253–374.

## Verify the certificates

The verifier program loads a certificate as a Python pickle file, interactively asks for a pair of indices, and then verifies the constraints corresponding to the user-specified range. Its usage message is the following.

```
usage: verifier.py [-h] [-p] [-v {1,2,3}] certificate

A simple flag algebras certificate verifier.

positional arguments:
  certificate          path of the pickle file

options:
  -h, --help          show this help message and exit
  -p, --partial        partial verification
  -v {1,2,3}, --verbose {1,2,3}
                        verbosity level
                        default: 1

examples:
$ python verify.py c5k4-bad-missing.pickle

$ python verify.py c5k4-bad-missing.pickle -p
Enter two integers in the range [1,28080] (e.g., '1 14040'): 1 10

$ python verifier.py c5k4-bad-missing.pickle -p -v 2
Enter two integers in the range [1,28080] (e.g., '1 14040'): 5 5
```

## Verifier specification

We work in the theory of 3-uniform hypergraphs, where every vertex is either red or blue. For a type  $\tau$  and integers  $m' \leq m$  such that  $2m' - |\tau| \leq m$ , we make the following definitions.

- $\mathcal{F}_m^\tau$  is the set of all flags with type  $\tau$  ( $\tau$ -flags) with  $m$  vertices in the theory. We also let  $\mathcal{F}_m = \mathcal{F}_m^\emptyset$ .
- $\mathbb{R}\mathcal{F}_m^\tau$  is the set of formal real linear combinations of flags from  $\mathcal{F}_m^\tau$ .
- For  $\tau$ -flags  $H_1, H_2 \in \mathcal{F}_{m'}^\tau$ , let  $H_1 \times H_2 = \sum_{G \in \mathcal{F}_{2m'-|\tau|}^\tau} d(H_1, H_2, G) G$ .
- $\mathcal{F}_{m'}^\tau \otimes \mathcal{F}_{m'}^\tau \in \left( \mathbb{R}\mathcal{F}_{2m'-|\tau|}^\tau \right)^{\mathcal{F}_{m'}^\tau \times \mathcal{F}_{m'}^\tau}$  is a symmetric matrix with lines indexed by  $\mathcal{F}_{m'}^\tau$  whose  $(H_1, H_2)$ -entry is  $H_1 \times H_2$ .
- $\llbracket \mathcal{F}_{m'}^\tau \otimes \mathcal{F}_{m'}^\tau \rrbracket_\tau \in \left( \mathbb{R}\mathcal{F}_{2m'-|\tau|}^\tau \right)^{\mathcal{F}_{m'}^\tau \times \mathcal{F}_{m'}^\tau}$  is the matrix obtained from  $\mathcal{F}_{m'}^\tau \otimes \mathcal{F}_{m'}^\tau$  by applying entry-wise the averaging operator. Each entry is a linear combination of flags from  $\mathcal{F}_{2m'-|\tau|}$ .

- For a flag  $F \in \mathcal{F}_m$ , we let  $M_F^{\tau, m} \in \mathbb{R}^{\mathcal{F}_{m'}^{\tau} \times \mathcal{F}_{m'}^{\tau}}$  be the real symmetric matrix obtained from  $\llbracket \mathcal{F}_{m'}^{\tau} \otimes \mathcal{F}_{m'}^{\tau} \rrbracket_{\tau}$  by applying entry-wise the  $p(\cdot, F)$  density operator.

We now fix:

- (i)  $T \in \mathbb{R}\mathcal{F}_m$ , a target linear combination of flags,
- (ii)  $\lambda \in \mathbb{R}$ , a bound,
- (iii)  $(\tau_1, n_1), \dots, (\tau_k, n_k)$ , a sequence of types and sizes,
- (iv)  $X^{\tau_1}, \dots, X^{\tau_k}$ , a sequence of square matrices.
- (v)  $e_1, \dots, e_p$ , a sequence of coefficients  $e_i \in \mathbb{R}$ .
- (vi)  $f^{(1)}, \dots, f^{(p)}$ , a sequence of elements  $f^{(i)} \in \mathbb{R}\mathcal{F}_m$ .

Then, we need to verify that:

$$\text{the matrices } X^{\tau_1}, \dots, X^{\tau_k} \text{ are positive semidefinite,} \quad (1)$$

and for all  $F \in \mathcal{F}_m$  and coefficients  $c_F \geq 0$ ,

$$\lambda - p(T, F) = \sum_{i \in [k]} \langle M_F^{\tau_i, m_i}, X^{\tau_i} \rangle + \sum_{i \in [p]} e_i p(f^{(i)}, F) + c_F. \quad (2)$$

The verification of (1) is done by attempting to decompose a matrix  $M = LDL^T$ , where  $L$  is a lower triangular matrix with 1's on the diagonal, and  $D$  is a diagonal matrix. If the decomposition reconstructs  $M$ , and all diagonal entries of  $D$  are non-negative, then we conclude that  $M$  is positive semidefinite.

Given that the verification of (2) may be computationally intensive, the program verifies a user-specified subset of  $\mathcal{F}_m$ . More precisely, given an ordering of the set

$$\mathcal{F}_m = \{F_1, F_2, \dots, F_{\ell}\}, \quad (3)$$

specified by the certificate, and a user-specified pair of indices  $i, j$ , the program verifies (2) for  $F_p$ , with  $i \leq p \leq j$ . By default, this range is  $[\ell]$ , i.e., the program completely verifies (2). If the verification fails at some point, the program stops and reports the failure.

A certificate is a Python pickle file containing a serialized dictionary with string keys. All numerical values in the certificate are `Fraction` objects. The structure of the dictionary is as follows:

- **"target"**: The target element in (i), given as a list  $(t_i)_{i \in [\ell]}$ , where  $T = t_1 F_1 + \dots + t_{\ell} F_{\ell}$ .
- **"result"**: The value in (ii).
- **"X matrices"**: List  $(X^{\tau_i})_{i \in [k]}$  of the matrices in (iv). Each matrix is given as a list representing a flattened matrix.
- **"e vector"**: List  $(e_i)_{i \in [p]}$  of coefficients in (v).
- **"positives"**: List  $(f^{(i)})_{i \in [p]}$  of positivity constraints in (vi). Each element  $f^{(i)}$  is given as a list  $(f_j^{(i)})_{j \in [\ell]}$ , where  $f^{(i)} = f_1^{(i)} F_1 + \dots + f_{\ell}^{(i)} F_{\ell}$ .
- **"base flags"**: List  $(F_i)_{i \in [\ell]}$  of the flags in (3). Each flag is given as a tuple with the following values:
  - Integer  $k$ , the number of vertices in the flag. The vertices of the flag are the integers  $0, 1, \dots, k-1$ .
  - Tuple  $\mathbf{t}$  of integers, the typed vertices of the flag in the labeling order. So,  $\mathbf{t}[0]$  is the vertex assigned to label 0, and so on.
  - Tuple or ordered pairs  $(\mathbf{r}, 1)$  identifying relations. The value  $\mathbf{r}$  is the name of the relation, one of the strings `edges`, `C0` or `C1`. The value 1 is a tuple identifying the elements of the relation. Each element of the relation is a tuple containing

the vertices in the relation. For example, this is a valid tuple of ordered pairs: ( ("edges", ((0, 1, 2)) ), ("C0", ((0), (1)) ), ("C1", (2)) ). The vertices in the relation C1 are the blue vertices. Every other vertex (i.e., those in C0) is red. The relations C0 and C1 are either both present, or both missing, in which case all the vertices are red.

- **"typed flags"**: Dictionary, where keys are pairs  $(\mathbf{m}, \mathbf{t})$ , where  $\mathbf{m}$  is an integer, and  $\mathbf{t}$  is a type  $\tau_i$  from (iii) in the flag format specified in the previous item. For a key  $(m_i, \tau_i)$ , its corresponding value is a list of the elements in  $\mathcal{F}_{m_i}^{\tau_i}$  in flag format.
- **"slack vector"**: List  $(c_{F_i})_{i \in [\ell]}$  of the non-negative slack coefficients in (2).
